# Supplementary material for: Role of disorder in finite-amplitude shear of a 2D jammed material
Source: arXiv:1410.2923 source file (2015-02-11)
Supplement: Supplementary file 1 [file supplemental.pdf]

# Supplementary Information for "Role of disorder in finite-amplitude shear of a 2D jammed material"

N. C. Keim and P. E. Arratia

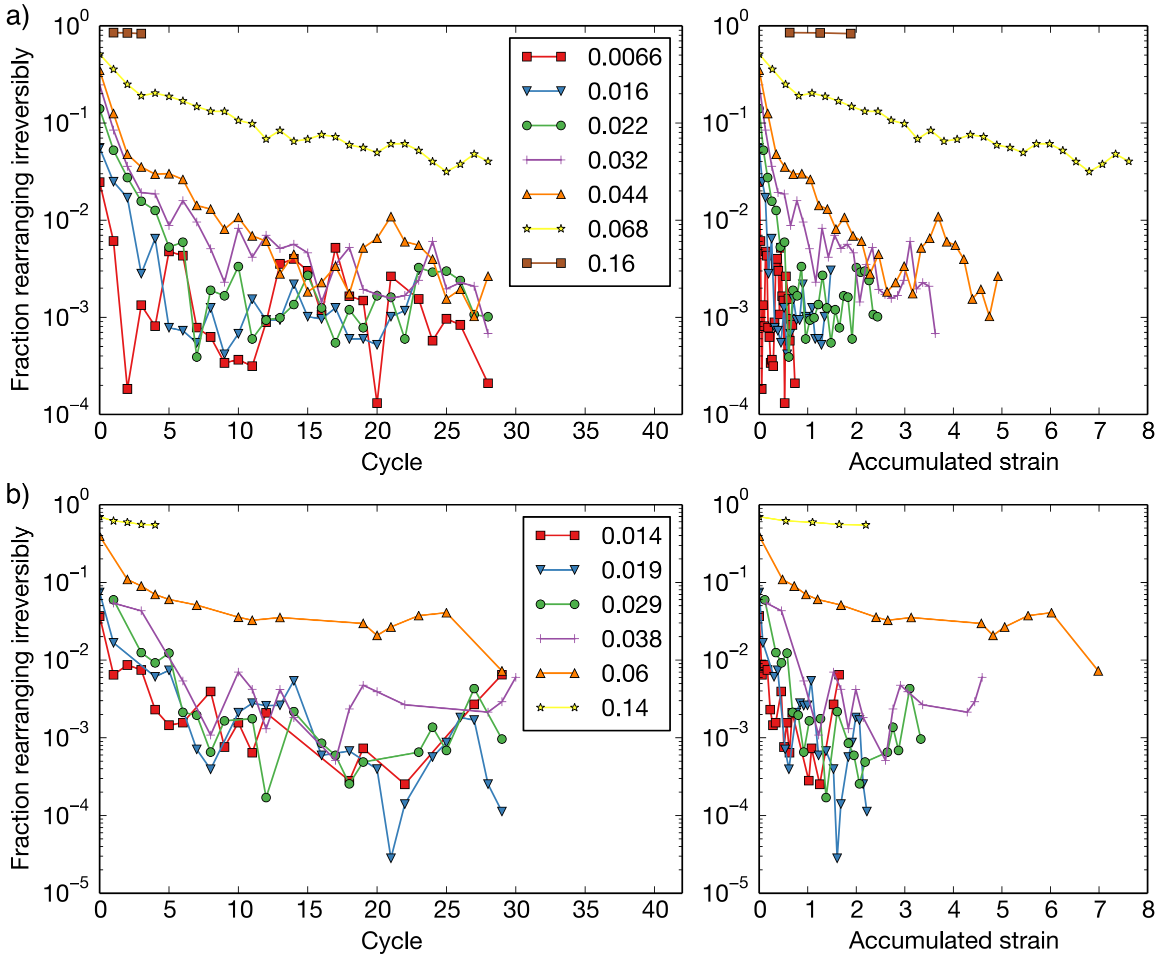


FIG. 1: Transient evolution of microstructure. For measurements of rearrangement activity in Fig. 3 of the main paper, we average over the steady state, which we define as beginning at the 15th cycle. **(a)** Left panel: Fraction of particles rearranging irreversibly in each cycle of movies of the bidisperse packing, at various $\gamma_0$. Right: Plotting the same data as a function of accumulated strain $\gamma_{\text{acc}} = 4\gamma_0 n$, where $n$ is the number of cycles, shows that the material requires more shearing to reach a steady state near the yielding transition. **(b)** Irreversible activity vs. cycle number for the monodisperse packing. Cycles with poor image quality were discarded; see Methods for details.

**Caption for Supplementary Movie 1**

**Left:** Video of a portion of the monodisperse packing, during a single cycle of deformation at $\gamma_0 = 0.038$. Particles that rearrange (total $D^2_{\mathrm{min}} \geq 0.015$) are highlighted in green; the images are cropped so that the large rearranging cluster is always centred. Legend at top shows global shear strain. **Right:** Tracked particle centres, coloured according to $D^2_{\mathrm{min}}$, which is computed relative to the beginning of the cycle. All rearrangements shown are reversed by the end of the cycle. The central rearranging cluster displays hysteresis: $D^2_{\mathrm{min}}$ rises significantly at $\gamma_{\mathrm{on}} \simeq 0.025$, but during reverse shearing does not fall until $\gamma_{\mathrm{off}} \simeq 0.005$. Note that just one video frame is included for every six in the original recording.
